# Supplementary material for: Using physics-based simulation towards eliminating empiricism in extraterrestrial terramechanics applications
Source: arXiv:2405.11001 source file (2024-05-17)
Supplement: Supplementary file 1 [file appendix.tex]

\section{Appendix: more about the parameter calibration of GRC-1 and GRC-3}
\label{sec:appendix}

\subsection{GRC-3}
\label{subsec:more_grc3}

\begin{figure}[h]
	\centering
	\begin{subfigure}{0.32\textwidth}
		\centering
		\includegraphics[width=2in]{calibration/grc3/Post_Mean_10000_samples_K_c.png}\\
		\includegraphics[width=2in]{calibration/grc3/Trace_10000_samples_K_c.png}\\
		\includegraphics[width=2in]{calibration/grc3/Post_10000_samples_K_c.png}
		\caption{$10000$}
	\end{subfigure}
	\begin{subfigure}{0.32\textwidth}
		\centering
		\includegraphics[width=2in]{calibration/grc3/Post_Mean_100000_samples_K_c.png}\\
		\includegraphics[width=2in]{calibration/grc3/Trace_100000_samples_K_c.png}\\
		\includegraphics[width=2in]{calibration/grc3/Post_100000_samples_K_c.png}
		\caption{$100000$}
	\end{subfigure}
	\begin{subfigure}{0.32\textwidth}
		\centering
		\includegraphics[width=2in]{calibration/grc3/Post_Mean_1000000_samples_K_c.png}\\
		\includegraphics[width=2in]{calibration/grc3/Trace_1000000_samples_K_c.png}\\
		\includegraphics[width=2in]{calibration/grc3/Post_1000000_samples_K_c.png}
		\caption{$1000000$}
	\end{subfigure}
	\caption{Posterior probability distribution and its kernel density estimation (KDE) and the sampling trace plots of four chains for the SCM parameter $K_c$ of GRC-3.} 
	\label{fig:posterior_grc3_Kc_comparison}
\end{figure}

\begin{figure}[h]
	\centering
	\begin{subfigure}{0.32\textwidth}
		\centering
		\includegraphics[width=2in]{calibration/grc3/Post_Mean_10000_samples_K_phi.png}\\
		\includegraphics[width=2in]{calibration/grc3/Trace_10000_samples_K_phi.png}\\
		\includegraphics[width=2in]{calibration/grc3/Post_10000_samples_K_phi.png}
		\caption{$10000$}
	\end{subfigure}
	\begin{subfigure}{0.32\textwidth}
		\centering
		\includegraphics[width=2in]{calibration/grc3/Post_Mean_100000_samples_K_phi.png}\\
		\includegraphics[width=2in]{calibration/grc3/Trace_100000_samples_K_phi.png}\\
		\includegraphics[width=2in]{calibration/grc3/Post_100000_samples_K_phi.png}
		\caption{$100000$}
	\end{subfigure}
	\begin{subfigure}{0.32\textwidth}
		\centering
		\includegraphics[width=2in]{calibration/grc3/Post_Mean_1000000_samples_K_phi.png}\\
		\includegraphics[width=2in]{calibration/grc3/Trace_1000000_samples_K_phi.png}\\
		\includegraphics[width=2in]{calibration/grc3/Post_1000000_samples_K_phi.png}
		\caption{$1000000$}
	\end{subfigure}
	\caption{Posterior probability distribution and its kernel density estimation (KDE) and the sampling trace plots of four chains for the SCM parameter $K_{\phi}$ of GRC-3.} 
	\label{fig:posterior_grc3_Kphi_comparison}
\end{figure}

\begin{figure}[h]
	\centering
	\begin{subfigure}{0.32\textwidth}
		\centering
		\includegraphics[width=2in]{calibration/grc3/Post_Mean_10000_samples_n.png}\\
		\includegraphics[width=2in]{calibration/grc3/Trace_10000_samples_n.png}\\
		\includegraphics[width=2in]{calibration/grc3/Post_10000_samples_n.png}
		\caption{$10000$}
	\end{subfigure}
	\begin{subfigure}{0.32\textwidth}
		\centering
		\includegraphics[width=2in]{calibration/grc3/Post_Mean_100000_samples_n.png}\\
		\includegraphics[width=2in]{calibration/grc3/Trace_100000_samples_n.png}\\
		\includegraphics[width=2in]{calibration/grc3/Post_100000_samples_n.png}
		\caption{$100000$}
	\end{subfigure}
	\begin{subfigure}{0.32\textwidth}
		\centering
		\includegraphics[width=2in]{calibration/grc3/Post_Mean_1000000_samples_n.png}\\
		\includegraphics[width=2in]{calibration/grc3/Trace_1000000_samples_n.png}\\
		\includegraphics[width=2in]{calibration/grc3/Post_1000000_samples_n.png}
		\caption{$1000000$}
	\end{subfigure}
	\caption{Posterior probability distribution and its kernel density estimation (KDE) and the sampling trace plots of four chains for the SCM parameter $n$ of GRC-3.} 
	\label{fig:posterior_grc3_n_comparison}
\end{figure}

\begin{figure}[h]
	\centering
	\begin{subfigure}{0.32\textwidth}
		\centering
		\includegraphics[width=2in]{calibration/grc3/Post_Mean_10000_samples_cohesion.png}\\
		\includegraphics[width=2in]{calibration/grc3/Trace_10000_samples_cohesion.png}\\
		\includegraphics[width=2in]{calibration/grc3/Post_10000_samples_cohesion.png}
		\caption{$10000$}
	\end{subfigure}
	\begin{subfigure}{0.32\textwidth}
		\centering
		\includegraphics[width=2in]{calibration/grc3/Post_Mean_100000_samples_cohesion.png}\\
		\includegraphics[width=2in]{calibration/grc3/Trace_100000_samples_cohesion.png}\\
		\includegraphics[width=2in]{calibration/grc3/Post_100000_samples_cohesion.png}
		\caption{$100000$}
	\end{subfigure}
	\begin{subfigure}{0.32\textwidth}
		\centering
		\includegraphics[width=2in]{calibration/grc3/Post_Mean_1000000_samples_cohesion.png}\\
		\includegraphics[width=2in]{calibration/grc3/Trace_1000000_samples_cohesion.png}\\
		\includegraphics[width=2in]{calibration/grc3/Post_1000000_samples_cohesion.png}
		\caption{$1000000$}
	\end{subfigure}
	\caption{Posterior probability distribution and its kernel density estimation (KDE) and the sampling trace plots of four chains for the SCM parameter $c$ of GRC-3.} 
	\label{fig:posterior_grc3_cohesion_comparison}
\end{figure}

\begin{figure}[h]
	\centering
	\begin{subfigure}{0.32\textwidth}
		\centering
		\includegraphics[width=2in]{calibration/grc3/Post_Mean_10000_samples_phi.png}\\
		\includegraphics[width=2in]{calibration/grc3/Trace_10000_samples_phi.png}\\
		\includegraphics[width=2in]{calibration/grc3/Post_10000_samples_phi.png}
		\caption{$10000$}
	\end{subfigure}
	\begin{subfigure}{0.32\textwidth}
		\centering
		\includegraphics[width=2in]{calibration/grc3/Post_Mean_100000_samples_phi.png}\\
		\includegraphics[width=2in]{calibration/grc3/Trace_100000_samples_phi.png}\\
		\includegraphics[width=2in]{calibration/grc3/Post_100000_samples_phi.png}
		\caption{$100000$}
	\end{subfigure}
	\begin{subfigure}{0.32\textwidth}
		\centering
		\includegraphics[width=2in]{calibration/grc3/Post_Mean_1000000_samples_phi.png}\\
		\includegraphics[width=2in]{calibration/grc3/Trace_1000000_samples_phi.png}\\
		\includegraphics[width=2in]{calibration/grc3/Post_1000000_samples_phi.png}
		\caption{$1000000$}
	\end{subfigure}
	\caption{Posterior probability distribution and its kernel density estimation (KDE) and the sampling trace plots of four chains for the SCM parameter $\phi$ of GRC-3.} 
	\label{fig:posterior_grc3_phi_comparison}
\end{figure}

\subsection{GRC-1}
\label{subsec:more_grc1}

\begin{figure}[h]
	\centering
	\begin{subfigure}{0.32\textwidth}
		\centering
		\includegraphics[width=2in]{calibration/grc1/Post_Mean_10000_samples_K_c.png}\\
		\includegraphics[width=2in]{calibration/grc1/Trace_10000_samples_K_c.png}\\
		\includegraphics[width=2in]{calibration/grc1/Post_10000_samples_K_c.png}
		\caption{$10000$}
	\end{subfigure}
	\begin{subfigure}{0.32\textwidth}
		\centering
		\includegraphics[width=2in]{calibration/grc1/Post_Mean_100000_samples_K_c.png}\\
		\includegraphics[width=2in]{calibration/grc1/Trace_100000_samples_K_c.png}\\
		\includegraphics[width=2in]{calibration/grc1/Post_100000_samples_K_c.png}
		\caption{$100000$}
	\end{subfigure}
	\begin{subfigure}{0.32\textwidth}
		\centering
		\includegraphics[width=2in]{calibration/grc1/Post_Mean_1000000_samples_K_c.png}\\
		\includegraphics[width=2in]{calibration/grc1/Trace_1000000_samples_K_c.png}\\
		\includegraphics[width=2in]{calibration/grc1/Post_1000000_samples_K_c.png}
		\caption{$1000000$}
	\end{subfigure}
	\caption{Posterior probability distribution and its kernel density estimation (KDE) and the sampling trace plots of four chains for the SCM parameter $K_c$ of GRC-1.} 
	\label{fig:posterior_grc1_Kc_comparison}
\end{figure}

\begin{figure}[h]
	\centering
	\begin{subfigure}{0.32\textwidth}
		\centering
		\includegraphics[width=2in]{calibration/grc1/Post_Mean_10000_samples_K_phi.png}\\
		\includegraphics[width=2in]{calibration/grc1/Trace_10000_samples_K_phi.png}\\
		\includegraphics[width=2in]{calibration/grc1/Post_10000_samples_K_phi.png}
		\caption{$10000$}
	\end{subfigure}
	\begin{subfigure}{0.32\textwidth}
		\centering
		\includegraphics[width=2in]{calibration/grc1/Post_Mean_100000_samples_K_phi.png}\\
		\includegraphics[width=2in]{calibration/grc1/Trace_100000_samples_K_phi.png}\\
		\includegraphics[width=2in]{calibration/grc1/Post_100000_samples_K_phi.png}
		\caption{$100000$}
	\end{subfigure}
	\begin{subfigure}{0.32\textwidth}
		\centering
		\includegraphics[width=2in]{calibration/grc1/Post_Mean_1000000_samples_K_phi.png}\\
		\includegraphics[width=2in]{calibration/grc1/Trace_1000000_samples_K_phi.png}\\
		\includegraphics[width=2in]{calibration/grc1/Post_1000000_samples_K_phi.png}
		\caption{$1000000$}
	\end{subfigure}
	\caption{Posterior probability distribution and its kernel density estimation (KDE) and the sampling trace plots of four chains for the SCM parameter $K_{\phi}$ of GRC-1.} 
	\label{fig:posterior_grc1_Kphi_comparison}
\end{figure}

\begin{figure}[h]
	\centering
	\begin{subfigure}{0.32\textwidth}
		\centering
		\includegraphics[width=2in]{calibration/grc1/Post_Mean_10000_samples_n.png}\\
		\includegraphics[width=2in]{calibration/grc1/Trace_10000_samples_n.png}\\
		\includegraphics[width=2in]{calibration/grc1/Post_10000_samples_n.png}
		\caption{$10000$}
	\end{subfigure}
	\begin{subfigure}{0.32\textwidth}
		\centering
		\includegraphics[width=2in]{calibration/grc1/Post_Mean_100000_samples_n.png}\\
		\includegraphics[width=2in]{calibration/grc1/Trace_100000_samples_n.png}\\
		\includegraphics[width=2in]{calibration/grc1/Post_100000_samples_n.png}
		\caption{$100000$}
	\end{subfigure}
	\begin{subfigure}{0.32\textwidth}
		\centering
		\includegraphics[width=2in]{calibration/grc1/Post_Mean_1000000_samples_n.png}\\
		\includegraphics[width=2in]{calibration/grc1/Trace_1000000_samples_n.png}\\
		\includegraphics[width=2in]{calibration/grc1/Post_1000000_samples_n.png}
		\caption{$1000000$}
	\end{subfigure}
	\caption{Posterior probability distribution and its kernel density estimation (KDE) and the sampling trace plots of four chains for the SCM parameter $n$ of GRC-1.} 
	\label{fig:posterior_grc1_n_comparison}
\end{figure}

\begin{figure}[h]
	\centering
	\begin{subfigure}{0.32\textwidth}
		\centering
		\includegraphics[width=2in]{calibration/grc1/Post_Mean_10000_samples_cohesion.png}\\
		\includegraphics[width=2in]{calibration/grc1/Trace_10000_samples_cohesion.png}\\
		\includegraphics[width=2in]{calibration/grc1/Post_10000_samples_cohesion.png}
		\caption{$10000$}
	\end{subfigure}
	\begin{subfigure}{0.32\textwidth}
		\centering
		\includegraphics[width=2in]{calibration/grc1/Post_Mean_100000_samples_cohesion.png}\\
		\includegraphics[width=2in]{calibration/grc1/Trace_100000_samples_cohesion.png}\\
		\includegraphics[width=2in]{calibration/grc1/Post_100000_samples_cohesion.png}
		\caption{$100000$}
	\end{subfigure}
	\begin{subfigure}{0.32\textwidth}
		\centering
		\includegraphics[width=2in]{calibration/grc1/Post_Mean_1000000_samples_cohesion.png}\\
		\includegraphics[width=2in]{calibration/grc1/Trace_1000000_samples_cohesion.png}\\
		\includegraphics[width=2in]{calibration/grc1/Post_1000000_samples_cohesion.png}
		\caption{$1000000$}
	\end{subfigure}
	\caption{Posterior probability distribution and its kernel density estimation (KDE) and the sampling trace plots of four chains for the SCM parameter $c$ of GRC-1.} 
	\label{fig:posterior_grc1_cohesion_comparison}
\end{figure}

\begin{figure}[h]
	\centering
	\begin{subfigure}{0.32\textwidth}
		\centering
		\includegraphics[width=2in]{calibration/grc1/Post_Mean_10000_samples_phi.png}\\
		\includegraphics[width=2in]{calibration/grc1/Trace_10000_samples_phi.png}\\
		\includegraphics[width=2in]{calibration/grc1/Post_10000_samples_phi.png}
		\caption{$10000$}
	\end{subfigure}
	\begin{subfigure}{0.32\textwidth}
		\centering
		\includegraphics[width=2in]{calibration/grc1/Post_Mean_100000_samples_phi.png}\\
		\includegraphics[width=2in]{calibration/grc1/Trace_100000_samples_phi.png}\\
		\includegraphics[width=2in]{calibration/grc1/Post_100000_samples_phi.png}
		\caption{$100000$}
	\end{subfigure}
	\begin{subfigure}{0.32\textwidth}
		\centering
		\includegraphics[width=2in]{calibration/grc1/Post_Mean_1000000_samples_phi.png}\\
		\includegraphics[width=2in]{calibration/grc1/Trace_1000000_samples_phi.png}\\
		\includegraphics[width=2in]{calibration/grc1/Post_1000000_samples_phi.png}
		\caption{$1000000$}
	\end{subfigure}
	\caption{Posterior probability distribution and its kernel density estimation (KDE) and the sampling trace plots of four chains for the SCM parameter $\phi$ of GRC-1.} 
	\label{fig:posterior_grc1_phi_comparison}
\end{figure}
